# Supplementary material for: Towards Real-World Burst Image Super-Resolution: Benchmark and Method
Source: arXiv:2309.04803 source file (2023-09-09)
Supplement: Supplementary file 2 [file supp_rgb_vis.pdf]

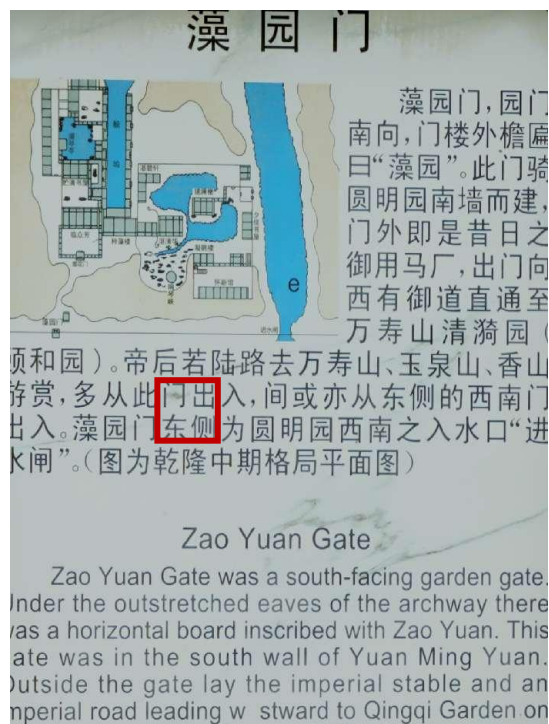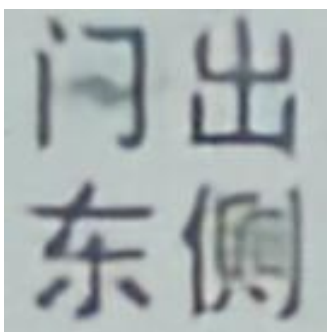

LP-KPN

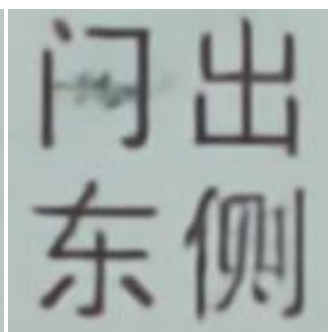

SwinIR

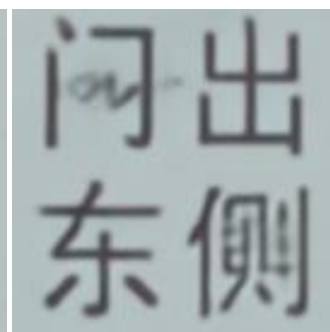

CDC

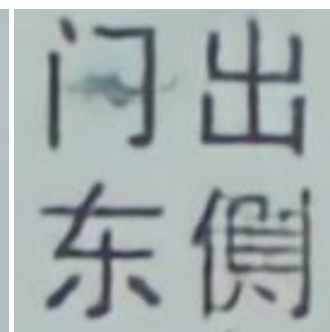

EDVR

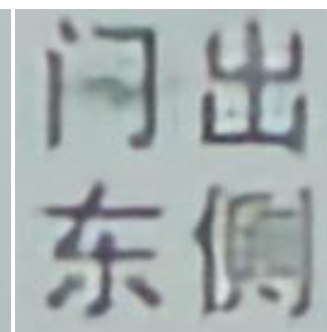

BasicVSR

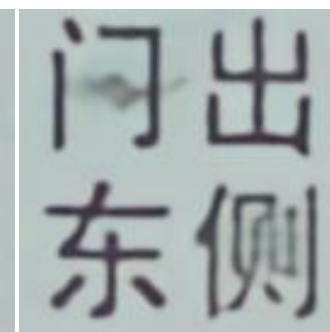

BasicVSR++

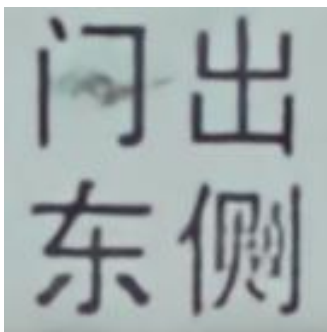

DBSR

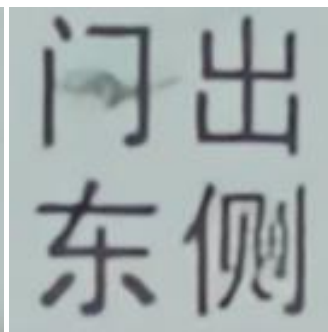

MFIR

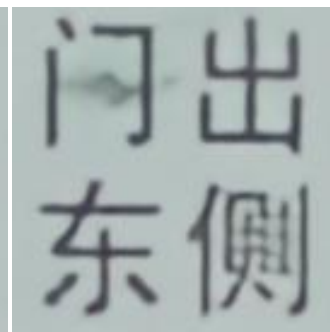

BSRT

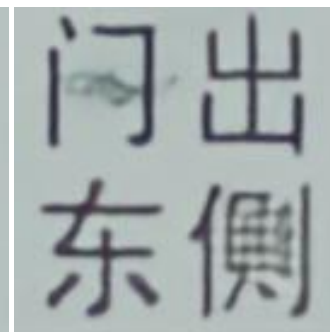

BIPNet

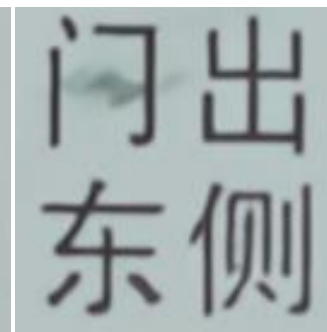

FBAnet(Ours)

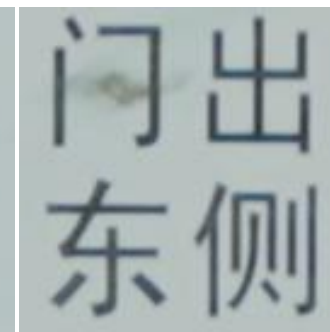

GT

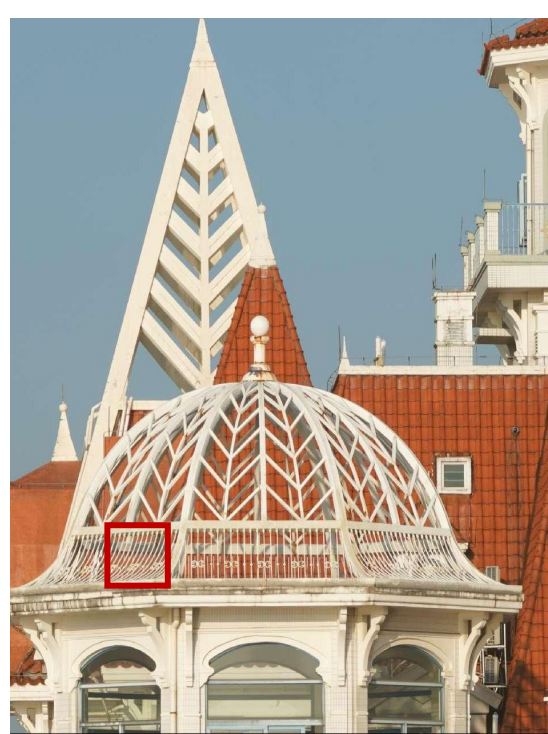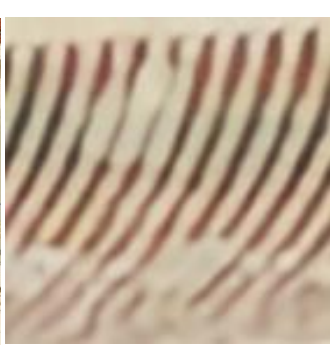

LP-KPN

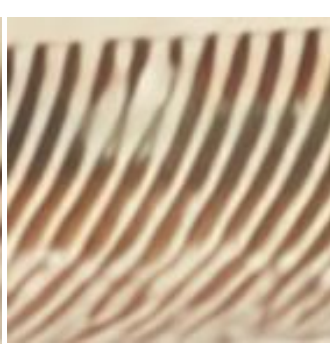

SwinIR

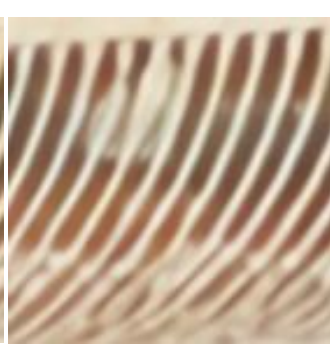

CDC

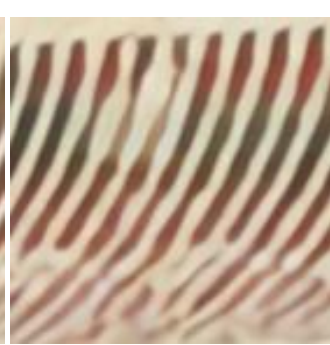

EDVR

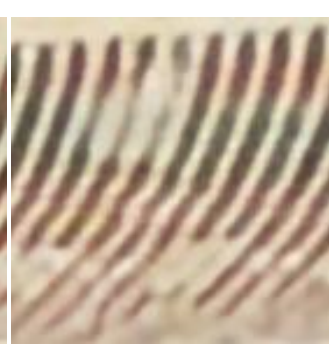

BasicVSR

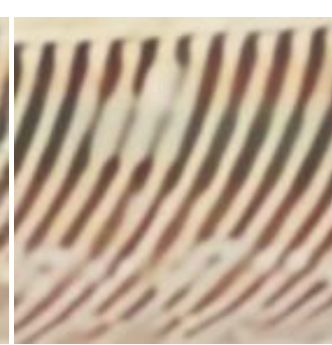

BasicVSR++

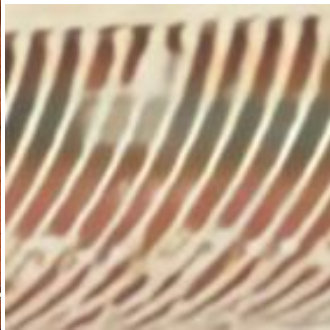

DBSR

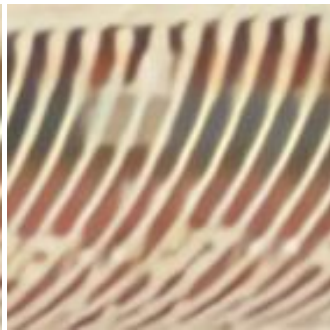

MFIR

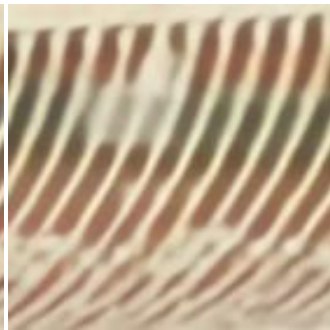

BSRT

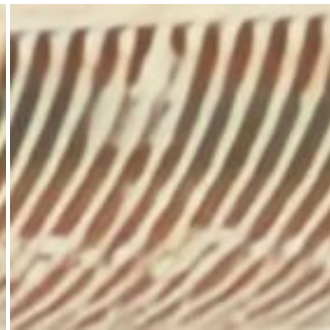

BIPNet

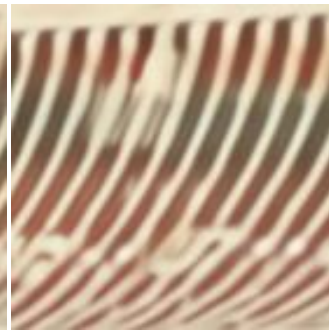

FBAnet(Ours)

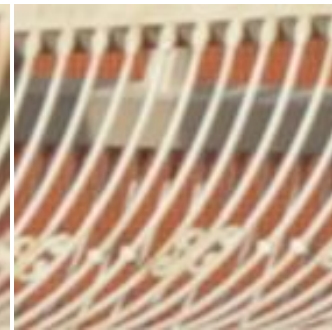

GT



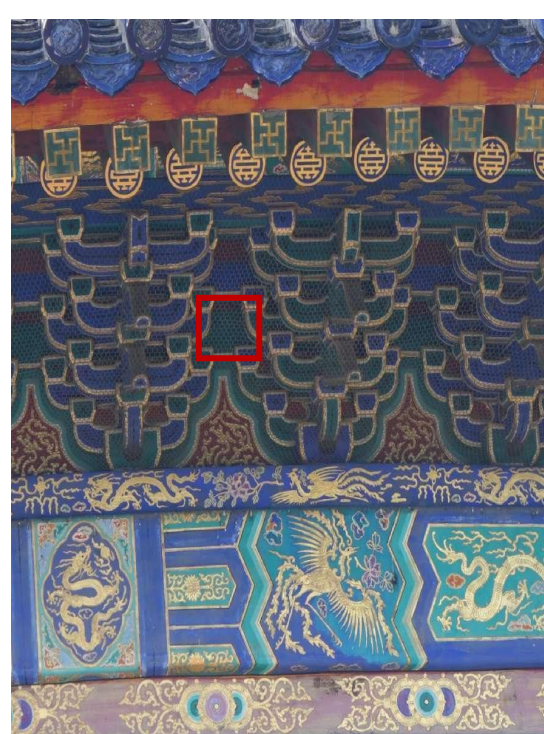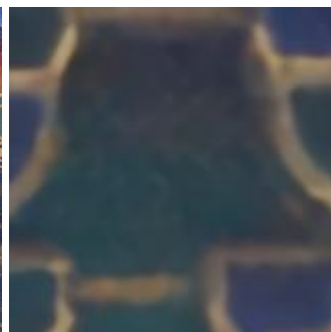

LP-KPN

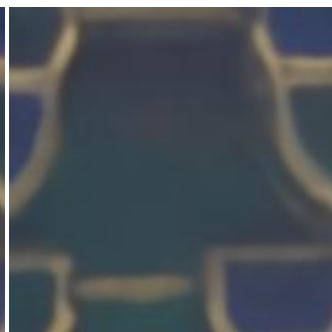

SwinIR

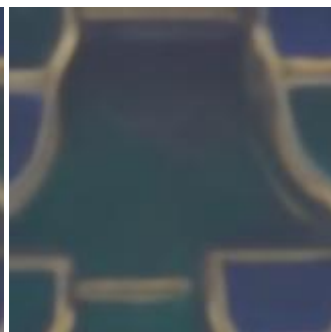

CDC

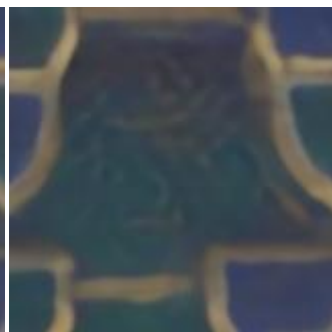

EDVR

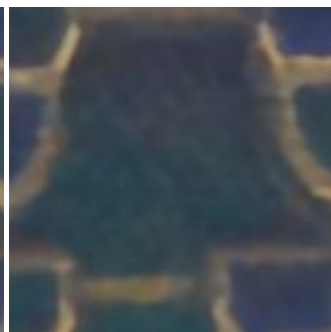

BasicVSR

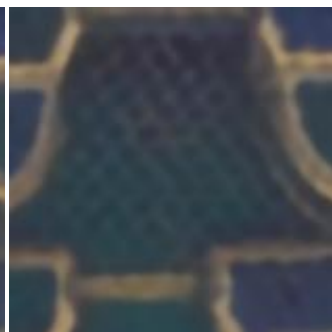

BasicVSR++

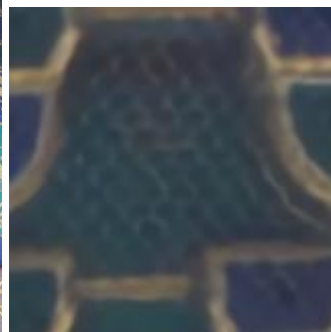

DBSR

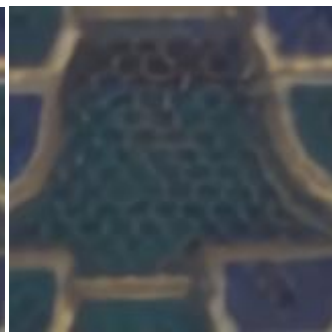

MFIR

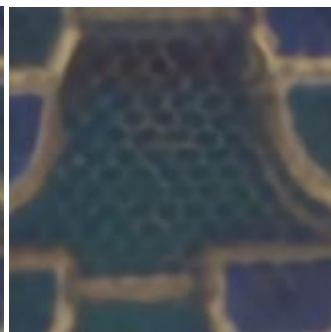

BSRT

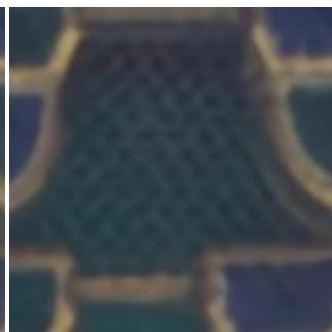

BIPNet

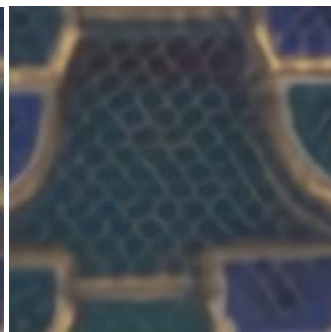

FBAnet(Ours)

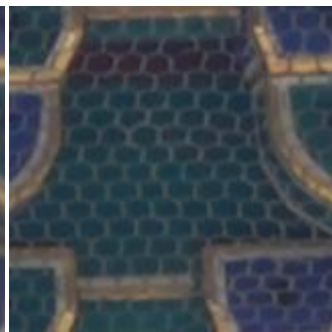

GT
